# Supplementary material for: Ranking with Slot Constraints
Source: arXiv:2310.17870 source file (2023-10-27)
Supplement: Supplementary file 1 [file appendix_illustration.tex]

The following toy example will illustrate our experiment setup. Suppose we have a list of 5 applicants $A = [A_1, \dots, A_5]$, in which $A_1, A_2$ belong to group 1 and $A_3, A_4, A_5$ belong to group 2. Group 1 has 2 allocated slots and group 2 has 1 allocated slot. In this case, $n = 5, m = 2 + 1 = 3$. \par

We can create an zero-valued $U$ sample matrix $U_i$ as shown in figure~\ref{fig:i-empty}. We connect applicant with their associated group's allocated slots in $U_i$ matrix, which is colored as red and cyan in figure~\ref{fig:i1}. We also sample from Bernoulli distribution for each unconnected (applicant, slot) pair in $U_i$ to determine if an edge should be added, where the new connected edges are colored as orange in figure~\ref{fig:i1}. \par

Suppose the applicant's qualification level array is $[0.5,\, 0.8,\, 0.3,\, 0.1,\, 1.0]$,
after the previous edge generation process, for each applicant, we will drop their edges with probability equal to 1 - (applicant's qualification level), as illustrated in figure~\ref{fig:i2}.

We will repeat the previous steps for $n_u$ times and stack all sampled $U_i$ to formulate the $\mathcal{U}$.

% \begin{figure}[!h]
%      \centering
%      \begin{subfigure}[b]{0.3\textwidth}
%          \centering
%          \includegraphics[width=\textwidth]{figures/simple_illustration-empty.png}
%          \caption{Initial Zero-valued $U_i$}
%          \label{fig:i-empty}
%      \end{subfigure}
%      \hfill     
%      \begin{subfigure}[b]{0.3\textwidth}
%          \centering
%          \includegraphics[width=\textwidth]{figures/simple_illustration-1.png}
%          \caption{$U_i$ After Edge Generation}
%          \label{fig:i1}
%      \end{subfigure}
%      \hfill
%      \begin{subfigure}[b]{0.3\textwidth}
%          \centering
%          \includegraphics[width=\textwidth]{figures/simple_illustration-2.png}
%          \caption{$U_i$ After Qualification Filtering}
%          \label{fig:i2}
%      \end{subfigure}
     
%      \caption{$U_i$ Sample Matrix Generation Process}
% \end{figure}

If $n_u = 1$, and $\mathcal{U}$ only contains the matrix in figure~\ref{fig:i2}, we can obtain the following results for our baseline and greedy bipartite matching algorithm\footnote{In case of a tie, we favor the lower indexed applicant here.}:

\begin{itemize}
    \item \textbf{Rank by Total Utilities}
    
    Total utilities $= [0,\, 3,\, 2,\, 0,\, 1]$, and the ranking is therefore $[A_2,\, A_3,\, A_5,\, A_1,\, A_4]$.

    \item \textbf{Rank by Total Utilities Normalized By Slot Competition}

    Normalized Total utilities $= [0,\, 1/2 + 1/2 + 1/2,\, 1/2 + 1/2,\, 0,\, 1/2] = [0,\, 3/2,\, 1,\, 0,\, 1/2]$, and the ranking is therefore $[A_2,\, A_5,\, A_3,\, A_1,\, A_4]$.

    \item \textbf{Rank by Qualification Level}
    Applicant's qualification level is $[0.5,\, 0.8,\, 0.3,\, 0.1,\, 1.0]$. The ranking is then $[A_5,\, A_2,\, A_1,\, A_3,\, A_4]$.

    \item \textbf{Rank by Random Permutation}
    A random permutation of the applicant list is  $[A_4,\, A_2,\, A_1,\, A_5,\, A_3]$, and this is the ranking.

    \item \textbf{Rank by Greedy Bipartite Matching}
    It is not hard to show greedy bipartite matching would produce a ranking as $[A_2,\, A_3,\, A_5,\, A_1,\, A_4]$, and the bipartite matching size is $[1,\, 2,\, 3,\, 3,\, 3]$. Notice that the bipartite matching size would reach the maximum as 3 after producing $[(A_2, S_1),\, (A_3, S_2),\, (A_5, S_3)]$ matching.

\end{itemize}
