# Supplementary material for: Ranking with Slot Constraints
Source: arXiv:2310.17870 source file (2023-10-27)
Supplement: Supplementary file 2 [file appendix_proof_submodular_monotone.tex]

\subsection{Proof for Theorem~\ref{thm:submodular} \label{sec:appendix-proof-submodular}}

\begin{proof}
    For monotonicity, as every matching from $C$ to $S$ is also a possible matching from $C \cup \{a\}$ to $S$, thus the size of the maximum matching from $C \cup \{x\}$ to $S$ must be at least the size of the maximum matching from $C$ to $S$. So we have 
    \begin{equation}
        \forall C \subseteq A, a \in A, \ |\text{MBM}(Q[C \cup \{ a \}, :])| \geq |\text{MBM}(Q[C, :])|
    \end{equation}

    For submodularity, we will show that $\forall C \subseteq A, \ a_1,\, a_2 \in A \setminus C$ such that $a_1 \neq a_2$, we have 
    \begin{multline}
        | \text{MBM}(C \cup \{a_2\}, Q)| - |\text{MBM} (C, Q)| \geq \\
        |\text{MBM} (C \cup \{a_1, a_2\}, Q)| - |\text{MBM} (C \cup \{a_1\}, Q)|. 
    \end{multline}

    Suppose $M_0$ is a maximal matching from $C$ to $S$, $M_1$ be $M_0$ after applying an augmenting path $P_1$ starting from $a_1$ and using nodes from $C \cup S \cup \{a_1\}$ (or if no such path exists, let $M_1 = M_0$), $M_{12}$ be $M_1$ after applying an augmenting path $P_{12}$ starting from $a_2$ and using nodes from $C \cup S \cup \{a_1, a_2\}$ (or if no such path exists, let $M_{12} = M_1$), and $M_2$ be $M_0$ after applying an augmenting path $P_2$ starting from $a_2$ and using nodes from $C \cup S \cup \{a_2\}$ (or if no such path exists, let $M_2 = M_0$). We want to show that 
    \begin{equation}
        |M_2| - |M_0| \geq |M_{12}| - |M_1| 
    \end{equation}
    
    The monotonicity says both the LHS and RHS is nonnegative, and with a single additional node on one side, the LHS and RHS can at most increase by 1. So the both LHS and RHS can be equal to either 0 or 1. It is sufficient to show that if $P_{12}$ exists, then an augmenting path starting from $a_2$ and using nodes from $C \cup S \cup \{a_2\}$, as $P_2$, indeed exists (LHS=1). 
    
    We first assume that $P_{12}$ exists; it traverses some vertices $[a_1, \ldots, a_t]$. If $P_1$ does not exist, then $P_{12}$ cannot have traversed through $a_1$ (due to the fact that augmenting paths alternate between matched and unmatched edges), so $P_{12}$ is one such desired augmenting path to $M_0$, starting from $a_2$, using only nodes from $C \cup S \cup \{a_2\}$. If $P_1$ does exist, suppose it traverses some vertices $b_1, \ldots, b_s$. If $P_1$ and $P_{12}$ do not share any vertices in common, then again $P_{12}$ is an augmenting path that satisfies the requirements. Otherwise, suppose $a_j = b_k$ is the first vertex where the paths overlap, and $a_{j'} = b_{k'}$ is the last vertex where the paths overlap. Since both paths start from unassigned nodes, we can splice the paths together to create a valid augmenting path $a_1, \ldots, a_j, b_k, \ldots, b_{k'}, a_{j'+1}, \ldots, a_r$, and this augmenting path also satisfies the requirements (starts from $a_2$ and only uses nodes from $C \cup S \cup \{a_2\}$, i.e. does not pass through $x_1$ due to the splicing construction -- in particular, applying $P_1$ causes $a_1$ to be matched to some slot $s$, so if $P_{12}$ hits $a_1$, it must first pass through $s$, but then $s = a_j = b_k$, so the splicing then reroutes the path along $P_1$ and the spliced path avoids $a_1$).
\end{proof}

\subsection{Proof for Lemma~\ref{lem:submodular-sum} \label{sec:appendix-proof-submodular-sum}}
\begin{proof}
    We know each individual objective $\text{\textbf{MBM}}(Q_i[C, :])$ is monotone and submodular from Theorem~\ref{thm:submodular}. Their summation is thus monotone and submodular.
\end{proof}

\subsection{Proof for Theorem~\ref{thm:exp}\label{sec:appendix-proof-exp}}
\begin{proof}
    Let $L(C) = 1-\frac{1}{m}\textrm{ExpMatch(C)}$ and $\hat{L}(C) = 1-\frac{1}{m}\textrm{AvgMatch(C)}$ (note assuming $n \geq m$). We have
    
    \begin{align*}
        L(\hat{C}) - L(C^*) &\leq |L(\hat{C}) - \hat{L}(\hat{C})| + |\hat{L}(\hat{C}) - \hat{L}(C^*)| + |\hat{L}(C^*) - L(C^*)| \\
        &\leq \frac{1}{e}(1-\hat{L}(C^*)) + 2\sup_C |L(C) - \hat{L}(C)| \\
        &\leq \frac{1}{e} + 2\sup_C |L(C) - \hat{L}(C)| \\
    \end{align*}
    
    Furthermore, for all $0<\delta<1/2$, with probability at least $1-\delta$, we have \[ |L(C) - \hat{L}(C)| \leq \sqrt{\frac{O(k\ln k) + \ln(2/\delta)}{2r}} \]
    
    due to Hoeffding + union bound across all possible $C$ (of which there are $k!$ possible values, and we have $\log k! = O(k \ln k)$). Combining gives that with probability at least $1-\delta$, we have
    
    \[ L(\hat{C}) - L(C^*) \leq \frac{1}{e} + \sqrt{\frac{O(k\ln k) + \ln(2/\delta)}{2r}}, \]
    
    i.e.
    
    \[ \textrm{ExpMatch}(C^*) - \textrm{ExpMatch}(\hat{C}) \leq \frac{m}{e} + m\sqrt{\frac{O(k\ln k) + \ln(2/\delta)}{2r}}, \]
\end{proof}
