# Supplementary material for: Ranking with Slot Constraints
Source: arXiv:2310.17870 source file (2023-10-27)
Supplement: Supplementary file 3 [file appendix_multilabel.tex]

\input{table/multilabel-brief-stats}
