# Supplementary material for: Ranking with Slot Constraints
Source: arXiv:2310.17870 source file (2023-10-27)
Supplement: Supplementary file 4 [file appendix_synthetic.tex]

\subsubsection{Simulated Experiment Framework}
