# Supplementary material for: Ranking with Slot Constraints
Source: arXiv:2310.17870 source file (2023-10-27)
Supplement: Supplementary file 5 [file obsolete.tex]

\begin{enumerate}
            
    Every applicant gets a uniform random qualification level from 0.2 to 0.3
    
    \item \textbf{Generate $U$ sample matrices}
    
    We repeat the following process 100 times to gather 100 $U$ samples:
    \begin{enumerate}
        \item Generate applicant-slot edge
        
        We first create a zero-valued biadjacency matrix $U_i \in \mathbf{0}^{n \times m}$. We connect each applicant's node with all of their assigned group's corresponding slot nodes. For slots from groups to which this applicant do not belong, we will connect an edge with probability 0.005 per group.
        
        Formally, suppose we have a $\text{GroupSlotListMap} = \{g_1: S_g^1, \dots, g_p: S_g^p\}$ that will map each group to the corresponding list of slot indices in each $U$ sample. If applicant $a$ has been assigned to group $g$, and group $g$ has slots that with their index list in $U_i$ as $S_g$, we will have 
        \vspace{-0.5em}\begin{align*}
            U_i[a,\, S_g] &= 1 \\
            \forall g_i \neq g \quad U_i[a,\, \text{GroupSlotListMap}[g_i]] &\sim \text{Bernoulli}(0.005)
        \end{align*}\vspace{-1em}

        \item Per applicant's qualification filtering
        
        With probability equal to 1 - ($a$'s qualification level), we will drop all of $a$'s edge. Formally, 
        
        \[U_i[a, :] \sim \text{Bernoulli}(Q[a]) * U_i[a, :]\]
        
    \end{enumerate}
    
    \item \textbf{Train-test split}
    
    We will use 80\% of $U$ samples as our training set to compute a static ranking, and after that we will evaluate each algorithm's output ranking on the 20\% test set.

    \vspace{1em}
    
\end{enumerate}
